# Supplementary material for: Complete crystal field calculation of Zeeman-hyperfine splittings in europium
Source: arXiv:2110.03896 source file (2021-10-28)
Supplement: Supplementary file 1 [file suppmat.pdf]

# Supplementary Materials

TABLE I. Experimental crystal field levels used for fitting and resulting calculated crystal field levels for the three $Eu^{3+}$ sites studied here ($cm^{-1}$).

| | $CaF_2$ $C_{4v}$ | | $CaF_2$ $C_{3v}$ | | $EuCl_3.6H_2O$ | |
|---|---|---|---|---|---|---|
| | Expt[a] | Calc | Expt[b] | Calc | Expt[c] | Calc |
| $^7F_0$ | 0 | −5 | 0 | −9 | 0 | −28 |
| $^7F_1$ | 307 | 315 | 217 | 223 | 301[d] | 276 |
| | 307 | 315 | 217 | 223 | 386[d] | 368 |
| | 456 | 484 | — | 865 | 423[d] | 410 |
| $^7F_2$ | 852 | 847 | 745 | 758 | — | 945 |
| | 971 | 956 | 745 | 758 | — | 970 |
| | 971 | 956 | 1219 | 1219 | — | 999 |
| | 1123 | 1135 | — | 1460 | — | 1012 |
| | 1261 | 1248 | — | 1460 | — | 1146 |
| $^7F_3$ | 1814 | 1802 | — | 1819 | — | 1797 |
| | 1814 | 1802 | — | 2010 | — | 1827 |
| | 1835 | 1824 | — | 2010 | — | 1846 |
| | 1953 | 1937 | — | 2071 | — | 1877 |
| | 1953 | 1937 | — | 2264 | — | 1908 |
| | 1977 | 1968 | — | 2324 | — | 1910 |
| | 2130 | 2118 | — | 2324 | — | 1913 |
| $^7F_4$ | 2510 | 2458 | — | 2784 | — | 2661 |
| | 2800 | 2771 | — | 2784 | — | 2671 |
| | 2800 | 2771 | — | 2819 | — | 2768 |
| | 2947 | 2927 | — | 3013 | — | 2865 |
| | 3006 | 2992 | — | 3013 | — | 2867 |
| | 3006 | 2992 | — | 3169 | — | 2872 |
| | 3089 | 3090 | — | 3432 | — | 2924 |
| | 3114 | 3123 | — | 3432 | — | 2951 |
| | 3156 | 3161 | — | 3452 | — | 3100 |
| $^7F_5$ | 3747 | 3744 | — | 3773 | — | 3747 |
| | 3829 | 3824 | — | 3837 | — | 3780 |
| | 3829 | 3824 | — | 3837 | — | 3797 |
| | 4020 | 3983 | — | 4053 | — | 3860 |
| | 4031 | 4040 | — | 4053 | — | 3893 |
| | 4035 | 4040 | — | 4131 | — | 3945 |
| | 4035 | 4046 | — | 4472 | — | 3949 |
| | 4115 | 4130 | — | 4475 | — | 3999 |
| | 4115 | 4130 | — | 4475 | — | 4024 |
| | 4183 | 4193 | — | 4773 | — | 4095 |
| | 4192 | 4201 | — | 4773 | — | 4111 |
| $^7F_6$ | 4866 | 4898 | — | 4842 | — | 4846 |
| | 4873 | 4911 | — | 5027 | — | 4847 |
| | 4873 | 4911 | — | 5027 | — | 4972 |
| | 4879 | 4924 | — | 5290 | — | 4972 |
| | 5150 | 5116 | — | 5290 | — | 4974 |
| | 5158 | 5148 | — | 5488 | — | 4992 |
| | 5158 | 5148 | — | 5586 | — | 4999 |
| | — | 5153 | — | 5746 | — | 5019 |
| | 5167 | 5157 | — | 5746 | — | 5082 |
| | 5184 | 5194 | — | 5892 | — | 5105 |
| | 5184 | 5194 | — | 5892 | — | 5129 |
| | — | 5379 | — | 5948 | — | 5220 |
| | — | 5379 | — | 5948 | — | 5221 |
| $^5D_0$ | 17288 | 17283 | 17422 | 17420 | 17250[d] | 17274 |

Continued on next page

TABLE I – continued from previous page

| | $CaF_2$ $C_{4v}$ | | $CaF_2$ $C_{3v}$ | | $EuCl_3.6H_2O$ | |
|---|---|---|---|---|---|---|
| | Expt[a] | Calc | Expt[b] | Calc | Expt[c] | Calc |
| $^5D_1$ | 19023 | 19012 | 19129 | 19110 | 18993[d] | 18998 |
| | 19023 | 19012 | 19129 | 19110 | 19003[d] | 19022 |
| | 19073 | 19077 | 19262 | 19292 | 19026[d] | 19035 |
| $^5D_2$ | 21455 | 21459 | 21586 | 21585 | 21455[d] | 21470 |
| | 21495 | 21591 | 21586 | 21585 | 21478[d] | 21477 |
| | 21537 | 21521 | 21673 | 21672 | 21480[d] | 21483 |
| | 21537 | 21521 | 21673 | 21672 | 21515[d] | 21499 |
| | — | 21526 | 21730 | 21716 | 21522[d] | 21510 |
| $^5D_3$ | 24335 | 24339 | — | 24419 | 24357 | 24340 |
| | 24335 | 24339 | — | 24479 | — | 24347 |
| | 24362 | 24355 | — | 24479 | — | 24362 |
| | 24371 | 24375 | — | 24535 | — | 24367 |
| | 24385 | 24384 | — | 24545 | — | 24378 |
| | 24397 | 24411 | — | 24545 | — | 24382 |
| | 24397 | 24411 | — | 24593 | — | 24394 |
| $^5L_6$ | — | 24924 | — | 24878 | 24988 | 24974 |
| | — | 24967 | — | 24878 | — | 24999 |
| | — | 24967 | — | 24916 | 25023 | 25014 |
| | — | 25019 | — | 24916 | 25054 | 25056 |
| | — | 25024 | — | 24932 | 25102 | 25097 |
| | — | 25053 | — | 25034 | 25114 | 25125 |
| | — | 25322 | — | 25470 | 25143 | 25148 |
| | — | 25333 | — | 25488 | 25200 | 25204 |
| | — | 25349 | — | 25488 | 25206 | 25211 |
| | — | 25349 | — | 25537 | 25267 | 25273 |
| | — | 25404 | — | 25720 | — | 25276 |
| | — | 25404 | — | 25720 | 25306 | 25331 |
| | — | 25452 | — | 25803 | 25327 | 25333 |
| $^5D_4$ | — | 27624 | — | 27853 | 27585 | 27589 |
| | — | 27627 | — | 27917 | 27602 | 27601 |
| | — | 27627 | — | 27917 | — | 27632 |
| | — | 27659 | — | 27942 | — | 27635 |
| | — | 27706 | — | 27946 | — | 27647 |
| | — | 27723 | — | 27946 | — | 27649 |
| | — | 27735 | — | 28018 | 27650 | 27656 |
| | — | 27738 | — | 28084 | — | 27680 |
| | — | 27738 | — | 28084 | 27690 | 27691 |
| $^3P_0$ | — | 32892 | — | 33081 | 32953 | 32907 |
| $\sigma$ | 18 | | 13 | | 15 | |

[a]Reference [1].
[b]Reference [2].
[c]Reference [3].
[d]Determined from experiment.

TABLE II. Mean free-ion parameters ($cm^{-1}$) for trivalent europium [4].

| $F^2$ | $F^4$ | $F^6$ | $\alpha$ | $\beta$ | $\gamma$ | $T^2$ | $T^3$ | $T^4$ | $T^6$ | $T^7$ | $T^8$ | $\zeta_{4f}$ | $M_{\text{tot}}$ | $P_{\text{tot}}$ |
|---|---|---|---|---|---|---|---|---|---|---|---|---|---|---|
| 82786 | 59401 | 42644 | 19.80 | −617 | 1460 | 370 | 40 | 40 | −330 | 380 | 370 | 1332 | 2.38 | 303 |

TABLE III. Symmetry element restrictions on the number of allowed $q$ values in the expansion of the crystal field [4].

| Symmetry element | Restrictions on $q$ |
|---|---|
| $C_n$ (parallel to the main axis) | $q$ is integer multiple of the rotation number $n$, but $q \leq k$ |
| $\sigma_h$ ($xy$-plane) | no terms with $q$ = even or $q = 0$ for odd k values; no terms $q$ = odd for even k values |
| $\sigma_v$ ($xz$-plane) | no imaginary terms |
| $C_2'$ (parallel to $x$-axis) | no terms with $q = 0$ for odd k values; no real terms with $k+\|q\|$ odd; no imaginary terms with $k+\|q\|$ even |
| $C_2'$ (parallel to $y$-axis) | no terms with $q = 0$ for odd k values; no real terms with $k+\|q\|$ odd; no imaginary terms with $k+\|q\|$ even |
| i (inversion through a center of symmetry) | no odd $k$ values |
| $S_n$ (parallel to main crystal axis) | no terms with $q = 0$ for odd k values; no terms with $q = n$-fold and $k+\|q\|$ odd; no terms with $q = \frac{(2x+1)n}{2}$, $(x = 0, 1, 2, \ldots)$ and $k+\|q\|$ even |

TABLE IV. Division of the 32 crystallographic point symmetry groups into the different symmetry classes and corresponding non zero crystal field parameters. Here the signs indicate whether parameters with positive or negative q are required [5].

| Class | | $B_0^2$ | $B_{\pm1}^2$ | $B_{\pm2}^2$ | $B_0^4$ | $B_{\pm1}^4$ | $B_{\pm2}^4$ | $B_{\pm3}^4$ | $B_{\pm4}^4$ | $B_0^6$ | $B_{\pm1}^6$ | $B_{\pm2}^6$ | $B_{\pm3}^6$ | $B_{\pm4}^6$ | $B_{\pm5}^6$ | $B_{\pm6}^6$ |
|---|---|---|---|---|---|---|---|---|---|---|---|---|---|---|---|---|
| Triclinic | $C_i$, $C_1$ | + | ± | ± | + | ± | ± | ± | ± | + | ± | ± | ± | ± | ± | ± |
| Monoclinic | $C_s$, $C_2$, $C_{2h}$ | + | | ± | + | | ± | | ± | + | | ± | | ± | | ± |
| Orthorhombic | $C_{2v}$, $D_2$, $D_{2h}$ | + | | + | + | | + | | + | + | | + | | + | | + |
| Tetragonal | $S_4$, $C_4$, $C_{4h}$ | + | | | + | | | | ± | + | | | | ± | | |
| | $D_{4h}$, $D_{2d}$, $C_{4v}$, $D_4$ | + | | | + | | | | + | + | | | | + | | |
| Trigonal | $S_6$ (= $C_{3i}$), $C_3$ | + | | | + | | | ± | | + | | | ± | | | ± |
| | $C_{3v}$, $D_3$, $D_{3d}$ | + | | | + | | | + | | + | | | + | | | + |
| Hexagonal | $C_6$, $C_{6h}$, $C_{3h}$ | + | | | + | | | | | + | | | | | | ± |
| | $D_6$, $D_{6h}$, $C_{6v}$, $D_{3h}$ | + | | | + | | | | | + | | | | | | + |
| Cubic | T, $T_h$ | | | | + | | | | + | + | | + | | + | | + |
| | O, $O_h$, $T_d$ | | | | + | | | | + | + | | | | + | | |
| Isoahedral | $I_h$ | | | | | | | | | + | | | | | + | |


[1] J. P. R. Wells and R. J. Reeves, Phys. Rev. B **64**, 035102 (2001).

[2] A. J. Silversmith, *High Resolution Laser Spectroscopy of Trivalent Europium Centers in Crystals*, Ph.D. thesis, Australian National University (1985).

[3] K. Binnemans and C. Görller-Walrand, J. Alloys Compd. **250**, 326 (1997).

[4] C. Görller-Walrand and K. Binnemans, in *Handb. Phys. Chem. Rare Earths*, Vol. 23 (Elsevier, 1996) Chap. 155, pp. 121–283.

[5] E. Bauer and M. Rotter, in *Prop. Appl. Complex Intermet.*, Vol. 2 (World Scientific, 2009) Chap. 5, pp. 183–248.
